# Supplementary material for: Dispersive gains enhance wireless power transfer with asymmetric resonance
Source: arXiv:2408.06913 source file (2024-08-13)
Supplement: Supplementary file 1 [file supp.pdf]

# Supplementary information: Dispersive gains enhance wireless power transfer with asymmetric resonance

Xianglin Hao[1,2†], Ke Yin[2,3†], Shiqing Cai[2†], Jianlong Zou[2], Ruibin Wang[2], Xikui Ma[2], Chi K. Tse[1*], Tianyu Dong[2*]

[1*]Department of Electrical Engineering, City University of Hong Kong, Hong Kong, China.
[2*]School of Electrical Engineering, Xi'an Jiaotong University, Xi'an, 710049, Shaanxi, China.
[3]College of Electronics and Information Engineering, Sichuan University, Chengdu, 610101, Sichuan, China.

*Corresponding author(s). E-mail(s): chitse@cityu.edu.hk; tydong@mail.xjtu.edu.cn;
Contributing authors: xianglhao2-c@my.cityu.edu.hk; yinke@scu.edu.cn; caisq1024@stu.xjtu.edu.cn; superzou@xjtu.edu.cn; 3121104276@stu.xjtu.edu.cn; maxikui@xjtu.edu.cn;
[†]These authors contributed equally to this work.

## 1 Theoretical analysis of asymmetric resonant systems

Fig. S1 shows a simplified schematic and basic circuit architecture of a dual coil wireless power transfer (WPT) system. In general, two analysis approaches are widely used for this type of WPT systems: one is based on intuitive coupled mode theory (CMT), and the other is based on electrical circuit theory. Within the coupled mode framework (Fig. S1**a**), the dynamics of the considered WPT system is characterized as $\mathrm{i}d\boldsymbol{a}/\mathrm{d}t = \boldsymbol{H}_{\mathrm{CMT}}\boldsymbol{a}$, where $\boldsymbol{a} = (a_1, a_2)^{\mathrm{T}}$ denotes the normal modes of the source and receiver resonator. When a valid Hamiltonian $\boldsymbol{H}_{\mathrm{CMT}}$ is modeled, the analysis of the system becomes straightforward and simple. According to CMT [1], the square of the ratio $|a_2/a_1|^2$ represents the ratio of the energy stored in the two resonators and the power transfer efficiency of the asymmetric resonant system can be obtained as

$$\eta_{\mathrm{CMT}} = \frac{\gamma_{\mathrm{load}}|a_2|^2}{\gamma_{\mathrm{sr}}|a_1|^2 + \gamma|a_2|^2} = \frac{\gamma_{\mathrm{load}}}{\gamma}\left(1 + \frac{\gamma_{\mathrm{sr}}}{\gamma}\Bigg/\left|\frac{a_2}{a_1}\right|^2\right)^{-1}. \tag{S1}$$

where $\gamma_{\mathrm{load}}$, $\gamma_{\mathrm{sr}}$ and $\gamma_{\mathrm{sr}}$ are the loss parameter of load resistors, the loss parameter of the receive resonator, and the intrinsic loss of the source resonator, respectively. In the case where CMT and Eq. (S1) apply [2, 3], increasing the energy storage ratio $|a_2/a_1|^2$ enables the improvement of the power transfer efficiency. Note that the power transfer efficiency of the parity-time (PT) symmetrical system is given by [3, 4]

$$\eta_{\mathrm{PT}} = \begin{cases} \dfrac{\gamma_{\mathrm{load}}}{\gamma}\left(1 + \dfrac{\gamma_{\mathrm{sr}}\gamma}{k^2}\right)^{-1}, & k < \gamma \\ \dfrac{\gamma_{\mathrm{load}}}{\gamma}\left(1 + \dfrac{\gamma_{\mathrm{sr}}}{\gamma}\right)^{-1}, & k \geq \gamma \end{cases} \tag{S2}$$

where $k$ is the coupling coefficient. In the strongly coupled region where $k \geq \gamma$, the efficiency is equivalent to the case of $|a_2/a_1|^2 = 1$ in Eq. (S1). Therefore, if the mode ratio is greater than one in Eq. (S1), the efficiency of the asymmetric resonant system can be higher than the maximum efficiency of the conventional PT-symmetric system. Moreover, by increasing the energy storage ratio $|a_2/a_1|^2$, the coefficient of loss parameter $\gamma_{\mathrm{rs}}$ in Eq. (S1) becomes small, indicating that the impact of the loss of the source resonator on the efficiency of the system is reduced. Since the energy storage ratio can be greater than one within our framework, it is possible to achieve a transfer efficiency comparable to that of the PT-symmetric architecture even when

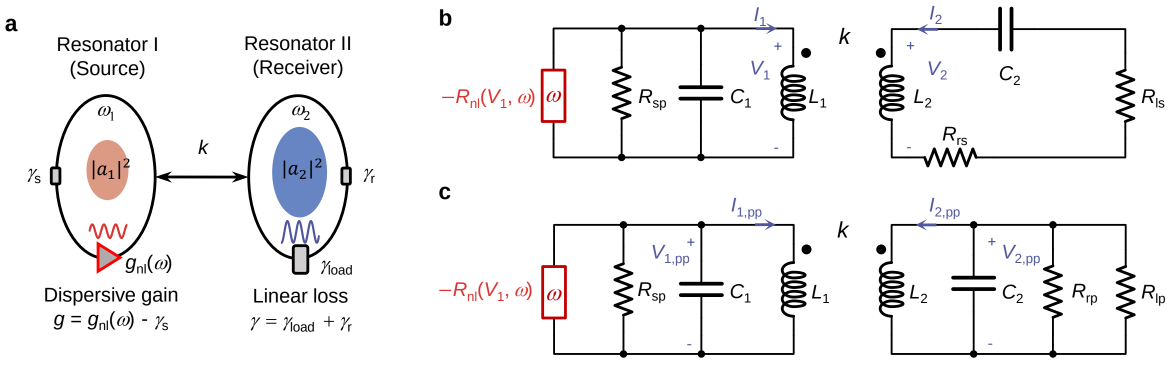


**Fig. S1 Illustration of wireless power transfer based on coupled resonators.** **a**, Schematic diagram of the coupled mode model of a dual-coil wireless power transfer system. Equivalent circuits of **b** parallel-series and **c** parallel-parallel wireless power transfer systems based on dispersion gain. Note that $R_{\mathrm{sp}}$ is the parallel equivalent resistance of the source resonator; and $R_{\mathrm{rp}}$ and $R_{\mathrm{rs}}$ are the parallel and series equivalent resistances of the receiving resonator, respectively. The load resistances in **b** and **c** are denoted by $R_{\mathrm{lp}}$ and $R_{\mathrm{ls}}$, respectively.

a source-side coil with a lower quality factor ($Q_{\mathrm{s}} \propto \gamma_{\mathrm{rs}}^{-1}$) is used, relaxing the quality factor requirement of the source coil in efficient WPT applications.

Although coupled mode theory provides a simple and powerful model that can effectively describe the physical mechanisms such as symmetry breaking, it ignores the microstructure of the resonators and the accuracy may be unsatisfactory in many cases [5]. In contrast, the method of applying circuit theory in analogy with the Schrödinger equation can model resonators more completely (though more complex) and depict the physical mechanism in asymmetric situations more clearly [6]. Moreover, with the introduction of the concept of normal mode by analogy to CMT [7], the analysis of stored energy can become quite intuitive. Now, by defining the wave function $\Psi = (V_1, V_2, I_1, I_2)^{\mathrm{T}}$ and $\tau = \omega_0 t$, the dynamic equation of the system can be described in Liouvillian form as $\mathrm{i}\mathrm{d}\Psi/\mathrm{d}\tau = \mathrm{i}\mathscr{L}\Psi$, where $\mathrm{i}\mathscr{L}$ can be interpreted as a non-Hermitian effective Hamiltonian $\boldsymbol{H}_{\mathrm{eff}} = \mathrm{i}\mathscr{L}$. For time-harmonic charge distributions $\Psi_n = A_n e^{\mathrm{i}\omega\tau}$, eigenfrequencies and normal modes for circuit systems can be derived from the eigenvalue equation $\mathrm{i}\omega\Psi = \mathscr{L}\Psi$. Defining the normal mode of resonators as $a_n = \sqrt{C_n/2}V_{Cn}$ where the subscripts $n = 1$ and $n = 2$ correspond to the source and receiver, respectively, one can then use the relationship between $V_2$, $I_1$, $I_2$, and $V_1$ to obtain the ratio of normal modes $a_2$ and $a_1$ substituting the eigenfrequencies into the dynamic equation. The ratio $a_2/a_1$ is a function of $\omega$, $k$ and $\gamma$, that is, $a_2/a_1 = f_{\mathrm{t}}(\omega, k, \gamma)$, where the specific form of $f_{\mathrm{t}}(\omega, k, \gamma)$ depends on the topology of the circuit. As shown in Fig. S1**b,c**, the inherent loss of a resonator can be modeled as equivalent parallel resistance or series resistance to calculate the power transfer efficiency of the system based on circuit theory, giving

$$\eta_{\mathrm{CT}} = \frac{P_{\mathrm{load}}}{P_{\mathrm{source}} + P_{\mathrm{receiver}} + P_{\mathrm{load}}} \tag{S3}$$

where the numerator $P_{\mathrm{load}}$ is the load power and the denominator is the total power injected into the resonator with $P_{\mathrm{source}}$ and $P_{\mathrm{receiver}}$ being the power loss in the source and receiver resonators, respectively.

To find $\mathscr{L}$, which is the key to analyzing this WPT system, we examine the circuit model of the coupled resonator system. For the parallel-series (PS) circuit shown in Fig. S1**b**, applying Kirchhoff's laws gives

$$I_1 + C_s \frac{\mathrm{d}V_1}{\mathrm{d}t} + \frac{V_1}{-R_{\mathrm{nl}}(V_1, \omega)} + \frac{V_1}{R_{\mathrm{sp}}} = 0, \tag{S4a}$$

$$V_2 + \frac{1}{C_r}\int_0^t I_2(\tau)\mathrm{d}\tau + I_2 R_{\mathrm{r}} = 0, \tag{S4b}$$

where $R_{\mathrm{r}} = R_{\mathrm{ls}} + R_{\mathrm{rs}}$. Moreover, the $I$–$V$ relationship of the inductors can be expressed as

$$\begin{pmatrix} V_1 \\ V_2 \end{pmatrix} = \begin{pmatrix} L_1 & M \\ M & L_2 \end{pmatrix} \begin{pmatrix} \mathrm{d}I_1/\mathrm{d}t \\ \mathrm{d}I_2/\mathrm{d}t \end{pmatrix} \tag{S5}$$

where $M$ is the mutual inductance between two resonator coils. In the following, we use the coupling parameter $k = M/(L_1 L_2)$ to represent the interaction of the two resonators. For simplicity, we assume $L_1 = L_2 = L$, $C_2 = C$, and $Z_{\mathrm{r}} = \sqrt{L/C}$, and denote the gain parameter by $g_{\mathrm{nl}}(V_1, \omega) = Z_{\mathrm{r}}/R_{\mathrm{nl}}(V_1, \omega)$ and the loss parameter by $\gamma = R_{\mathrm{r}}/Z_{\mathrm{r}}$. Also, the intrinsic loss parameter of the source resonator is $\gamma_{\mathrm{s}} = Z_{\mathrm{r}}/R_{\mathrm{sp}}$. Note that $\gamma_{\mathrm{sr}} = \chi\gamma_{\mathrm{s}}$ in Eq. (S1). When the quality factor ($Q_{\mathrm{s}} = 1/\gamma_{\mathrm{s}}$) of the source resonator is

large enough, we have $\gamma_s \approx 0$ and Eq. (S6) can be simplified to Eq. (1) of the main paper. Recasting Eq. (S4) and Eq. (S5) leads to the Liouvillian formalism of the dynamic equation $\mathrm{d}\Psi/\mathrm{d}\tau = \mathscr{L}_{\mathrm{PS}}\Psi$, where $\mathscr{L}_{\mathrm{PS}}$ is

$$\mathscr{L}_{\mathrm{PS}} = \begin{pmatrix} [g_{\mathrm{nl}}(V_1,\omega)-\gamma_s]\,\chi & 0 & -\chi Z_{\mathrm{r}} & 0 \\ \dfrac{k}{1-k^2}\gamma & -\dfrac{1}{1-k^2}\gamma & 0 & -Z_{\mathrm{r}} \\ \dfrac{1}{1-k^2}\dfrac{1}{Z_{\mathrm{r}}} & -\dfrac{k}{1-k^2}\dfrac{1}{Z_{\mathrm{r}}} & 0 & 0 \\ -\dfrac{k}{1-k^2}\dfrac{1}{Z_{\mathrm{r}}} & \dfrac{1}{1-k^2}\dfrac{1}{Z_{\mathrm{r}}} & 0 & 0 \end{pmatrix}. \tag{S6}$$

Here, $\chi = C_2/C_1$ is the asymmetric parameter, which can be designed according to application requirements. Consequently, the dynamics can be studied by the characteristic equation $\det(\omega\mathbb{I}_4 - \mathrm{i}\mathscr{L}_{\mathrm{PS}}) = 0$. For the PS circuit system considered, complex eigenfrequencies and their corresponding steady-state gains will evolve with $k$ and $\chi$, unveiling three distinct regimes of system behavior, as illustrated in Eq. (4) and Fig. 3 of the main paper. The intrinsic loss of the resonators can be modeled as $R_{\mathrm{sp}}$ and $R_{\mathrm{rs}}$, as shown in Fig. S1**b**, giving $P_{\mathrm{load}} = I_2^2 R_{\mathrm{ls}}/2$ for the load power received and $P_{\mathrm{source}} = V_1^2/(2R_{\mathrm{sp}})$ and $P_{\mathrm{receiver}} = I_2^2 R_{\mathrm{rs}}/2$ for the loss. Therefore, the power transfer efficiency Eq. (S3) of the PS circuit can be expressed as

$$\eta_{\mathrm{PS}} = \frac{R_{\mathrm{ls}}}{R_{\mathrm{ls}}+R_{\mathrm{rs}}}\left[1+\frac{1}{(R_{\mathrm{ls}}+R_{\mathrm{rs}})R_{\mathrm{sp}}}\left|\frac{I_2}{V_1}\right|^{-2}\right]^{-1}. \tag{S7}$$

It is evident the power transfer efficiency of the PS circuit can be improved by increasing the ratio $|I_2/V_1|$, which can be obtained from the output characteristic of the PS topology, i.e., $I_2/V_1 = -\mathrm{i}k\omega\omega_0/\left\{Z_{\mathrm{r}}\left[\mathrm{i}\gamma\omega\omega_0 + (k^2-1)\omega^2+\omega_0^2\right]\right\}$.

# 2 Comparison of different resonant topologies

## 2.1 Parallel-parallel topology

Similar to Eq. (S4)–Eq. (S6), analysis of the parallel-parallel (PP) circuit shown in Fig. S1**c** can be performed. Defining the wave function $\Psi = (V_{1,\mathrm{pp}}, V_{2,\mathrm{pp}}, I_{1,\mathrm{pp}}, I_{2,\mathrm{pp}})^{\mathrm{T}}$, the Liouvillian operator of the PP topology can be derived as

$$\mathscr{L}_{\mathrm{PP}} = \begin{pmatrix} \chi g_{\mathrm{nl}}(V_1,\omega) & 0 & -\chi Z_{\mathrm{r}} & 0 \\ 0 & -\gamma & 0 & -Z_{\mathrm{r}} \\ \dfrac{1}{1-k^2}\dfrac{1}{Z_{\mathrm{r}}} & -\dfrac{k}{1-k^2}\dfrac{1}{Z_{\mathrm{r}}} & 0 & 0 \\ -\dfrac{k}{1-k^2}\dfrac{1}{Z_{\mathrm{r}}} & \dfrac{1}{1-k^2}\dfrac{1}{Z_{\mathrm{r}}} & 0 & 0 \end{pmatrix}. \tag{S8}$$

The characteristic equation $\det(\mathscr{L}_{\mathrm{PP}} - \mathrm{i}\omega\mathbb{I}_4) = 0$ can be expanded as

$$\omega^4 - \frac{1+\chi-\gamma g_{\mathrm{nl}}(V_1,\omega)(1-k^2)\chi}{1-k^2}\omega^2 + \frac{\chi}{1-k^2} + \mathrm{i}\left\{[g_{\mathrm{nl}}(V_1,\omega)\chi-\gamma]\,\omega^3 - \frac{[g_{\mathrm{nl}}(V_1,\omega)-\gamma]\,\chi}{1-k^2}\omega\right\} = 0, \tag{S9}$$

solving which gives the steady-state solution for $\omega$.

We first consider the case where the gain element is nondispersive, i.e., $g_{\mathrm{nl}}(V_1,\omega) = g_{\mathrm{src}}(V_1)$. Putting the imaginary part of the characteristic equation Eq. (S9) to zero, the steady-state gain coefficient required for the nondispersive gain element can be obtained as

$$g_{\mathrm{PP}}^{\mathrm{non}} = \frac{\chi-(1-k^2)\omega^2}{\chi-(1-k^2)\omega^2\chi}\gamma. \tag{S10}$$

However, for an ideal dispersive device with gain equal to $g_{\mathrm{nl}}(V_1,\omega) = g_{\mathrm{src}}(V_1)/\omega^2$, the steady-state gain required becomes

$$g_{\mathrm{PP}}^{\mathrm{dis}} = g_{\mathrm{PP}}^{\mathrm{non}}\omega^2. \tag{S11}$$

Substituting the saturation gain required Eq. (S10) into the real part of the characteristic equation Eq. (S9), we can obtain the characteristic equation $\omega^6 + c_1\omega^4 + c_2\omega^2 + c_3 = 0$, where $c_1 = \gamma^2 - (\chi+2)(1-k^2)$, $c_2 = \{[2-\gamma^2-(1-\gamma^2)k^2]\chi+1\}/(1-k^2)^2$, and $c_3 = -\chi/(1-k^2)^2$; and the steady-state eigenfrequency can be derived by using the Cardano formula. Consequently, by

substituting each pair of eigenfrequencies back into Eq. (S10), the corresponding saturation gain required of each mode can be further obtained. Fig. S2**a** illustrates the eigenfrequency as a function of $k$ when the frequency detuning parameter (a.k.a. asymmetry factor) $\chi = 4/3$, and the saturation gain evolution of non-dispersive and dispersive system are presented in Fig. S2**b** and Fig. S2**c** respectively. In a non-dispersive detuned PT-symmetric WPT system, $\omega_1$ is always the real mode with the smallest saturation gain, which is the steady-state mode, as shown in Fig. S2**b**. However, in a dispersive detuned WPT system, since the gain interleaving will occur as the coupling coefficient $k$ increases, the steady-state mode, i.e., the mode with the smallest saturation gain, will switch from $\omega_1$ to $\omega_2$, resulting in a frequency jump at the intersection point, as shown in Fig. S2**c**.

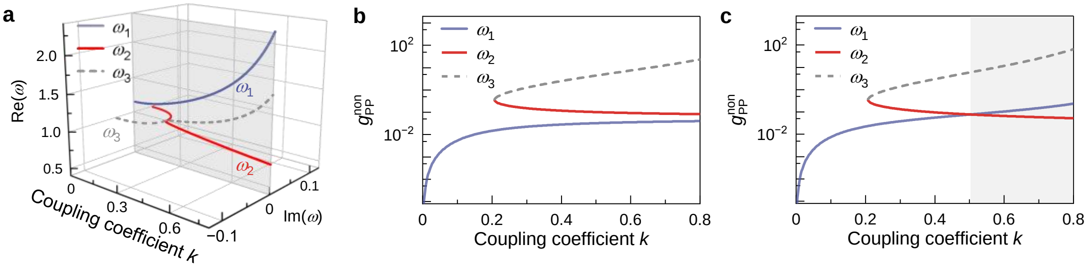


**Fig. S2 Parallel-parallel circuit with asymmetric parameters. a** Eigenfrequency and **b,c** saturation gain of (**b**) non-dispersive and (**c**) dispersive PT-symmetric WPT system with PP topology as a function of the coupling parameter $k$ when $\chi = 4/3$.

The normal mode of the resonators can be calculated by $a_n = V_{n,\text{pp}}\sqrt{C_n/2}$ with subscripts $n = 1$ and $n = 2$ corresponding to the source and receiver, respectively. According to the eigenfrequencies and the dynamic equation, the ratio of the voltage amplitude can be calculated by $V_{2,\text{pp}}/V_{1,\text{pp}} = k\omega_0^2/\left[(k^2-1)\omega^2 + \omega_0^2 + \mathrm{i}\gamma(k^2-1)\omega\omega_0\right]$ and shown in Fig. S3**a,b**. Fig. S3**c** and Fig. S3**d** plot the energy storage ratios $|a_2/a_1|^2 = C_2V_{2,\text{pp}}^2/(C_1V_{1,\text{pp}}^2)$ for the non-dispersive and dispersive systems, respectively. Using the energy storage ratio, the efficiencies can be further calculated using Eq. (S1), which can also be calculated using circuit theory. According to Eq. (S3), the power should be carefully calculated to obtain the transfer efficiency. For the PP topology, the power delivered to the load resistor is $P_{\text{load}} = V_{2,\text{pp}}^2/(2R_{\text{lp}})$, while the power losses of the source coil and the receiving coil are $P_{\text{source}} = V_{1,\text{pp}}^2/(2R_{\text{sp}})$ and $P_{\text{receiver}} = V_{2,\text{pp}}^2/(2R_{\text{rp}})$, respectively. As a result, the power transfer efficiency of the PP circuit can be expressed as

$$\eta_{\text{PP}} = \frac{R_{\text{rp}}||R_{\text{lp}}}{R_{\text{lp}}}\left(1 + \frac{R_{\text{rp}}||R_{\text{lp}}}{R_{\text{sp}}}\Bigg/\left|\frac{V_{2,\text{pp}}}{V_{1,\text{pp}}}\right|^2\right)^{-1}, \tag{S12}$$

where $R_{\text{rp}}||R_{\text{lp}} = (1/R_{\text{rp}} + 1/R_{\text{lp}})^{-1}$. In fact, Eq. (S12) and Eq. (S3) are equivalent. In PT-symmetric systems, the voltage ratio always corresponds to the strongly coupled case (symmetric phase). Compared to PT-symmetric systems, the voltage ratio in the dispersion-gain system is always better, i.e., greater than one in the strongly coupled region, as shown in Fig. S3**a,b**. Therefore, the power transfer efficiency of a PP circuit system with dispersive gain in this paper is higher than that of the PT-symmetric system. Fig. S3**c–f** compares the energy storage ratios and power transfer efficiencies between the non-dispersive and dispersive system. For a non-dispersive WPT system, $\omega_1$ is the steady-state mode and the steady-state energy storage ratio and efficiency are equivalent to the results corresponding to $\omega_1$. However, for a dispersive system, an abrupt increase in the energy storage ratio and efficiency will occur because of the steady-state mode transition.

## 2.2 Parallel-series topology

For a non-dispersive WPT system with PS topology, the saturation gain $g_{\text{nl}}(V_1,\omega)$ is only voltage-dependent and becomes $g_{\text{src}}(V_1)$. The steady-state saturation gain required can be derived as

$$g_{\text{PS}}^{\text{non}} = \frac{\gamma(\chi-\omega^2)}{(k^2-1)\,\omega^2\chi + \chi}. \tag{S13}$$

Since the steady-state frequencies of a PT-symmetric WPT system with non-dispersive and dispersive gain satisfy the same characteristic equation, the eigenfrequencies of the two systems show the same evolution, as shown in Fig. 3d of the main paper. Fig. S4**a** and Fig. S4**b** compare the evolution of the required saturation gain of non-dispersive system and dispersive system when $\chi = 4/3$. Unlike Fig. S2**b** and similar to Fig. S2**c**, the asymmetric topology itself causes the interleaving of the saturation gain. However, the PS topology with dispersive gain exhibits a smaller coupling parameter at the intersection point, thus increasing the coupling range for the high-efficiency mode $\omega_2$ to reach the steady state.

As in the case of the PP topology, the normal mode of the source and receiver resonators can be defined as $a_n = V_{Cn}\sqrt{C_n/2}$ with subscripts $n = 1$ and $n = 2$ corresponding to the source and receiver, respectively, where $V_{C1} = V_1$ and

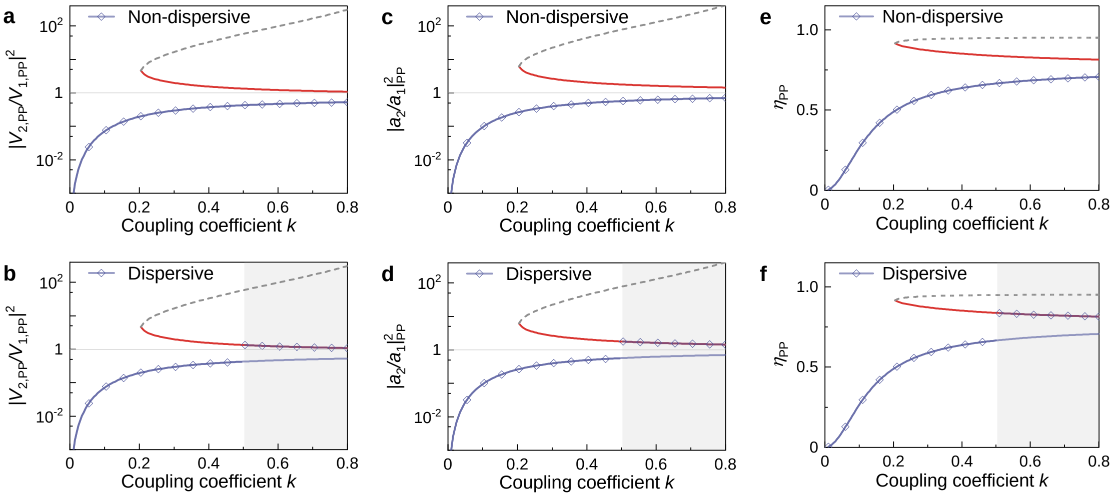


**Fig. S3 Performance comparison of parallel-parallel (PP) topology circuits using dispersive and non-dispersive gain. a,b** The ratio of the square of the voltage amplitude $|V_{2,\mathrm{pp}}/V_{1,\mathrm{pp}}|^2$, **c,d** energy storage ratio $|a_2/a_1|^2$, and **e,f** efficiency of non-dispersive and dispersive PT-symmetric WPT system with PP topology as a function of the coupling parameter $k$ when $\chi = 4/3$.

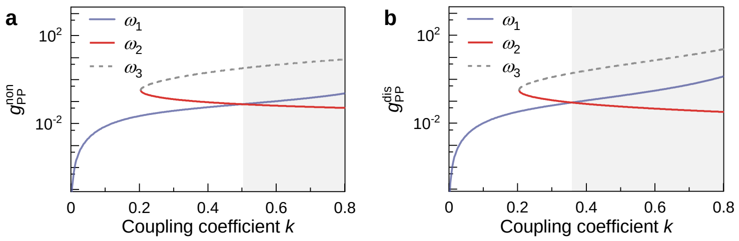


**Fig. S4 Comparison of the steady-state required gain of parallel-series (PS) circuits based on non-dispersive and dispersive devices.** Steady state required gain evolution of **a** non-dispersive and **b** dispersive asymmetric WPT system with PS topology versus the coupling parameter $k$ when $\chi = 4/3$.

$V_{C2} = -V_2 - I_2(R_{\mathrm{ls}} + R_{\mathrm{rs}})$. Since the voltage amplitude ratio between the compensation capacitors can be calculated by $V_{C2}/V_{C1} = -k\omega_0^2/\left[(k^2-1)\omega^2 + \omega_0^2 + \mathrm{i}\gamma\omega\omega_0\right]$, one can also derive the energy storage ratio $|a_2/a_1|^2$ of the WPT system with the PS topology can also be derive. Fig. S5**a** and Fig. S5**b** plot the energy storage ratios of non-dispersive and dispersive systems, respectively. Interestingly, a coupling range exhibits where the system stabilizes in the mode with higher energy storage ratio, which is due to the smaller coupling coefficient at the gain intersection point of a dispersive system compared to non-dispersive system. Furthermore, unlike a nondispersive system in which the energy storage ratio varies continuously, the energy storage ratio of the dispersive system will abruptly increase at the gain intersection point and then gradually decrease. Moreover, the dispersive system can work in the higher efficiency mode over a small coupling interval, resulting in a longer coupling range with high efficiency, as shown in Fig. S5**c** and Fig. S5**d**.

## 2.3 Comparison and discussion

Based on the above analysis, the power transfer efficiency can be improved by introducing a dispersive gain into a conventional PT symmetric system in either the PP topology or the PS topology. In addition, the efficiency of the dispersive system is higher than non-dispersive system in the entire strong coupling region for the PP topology. For the PS topology, the system works only in the higher-efficiency mode within a coupling interval of the strong coupling region. Moreover, gain interleaving is introduced by either asymmetric topology or dispersive gain.

Note that the dispersive gain element introduces not only the saturation effect but also the nonlinearity in the frequency domain into the non-Hermitian system; and the fusion of the two types of nonlinear effects may further reveal unknown and more complex harmonic dynamics in non-Hermitian physics. In addition, it has been known that high-order topology can also be used to design steady-state modes of the system [8, 9]. The integration of topology and frequency-domain nonlinearity may give rise to a novel non-Hermitian topology and dispersion engineering to address existing energy and information transfer issues, providing new ways for developing power transfer and sensing techniques.

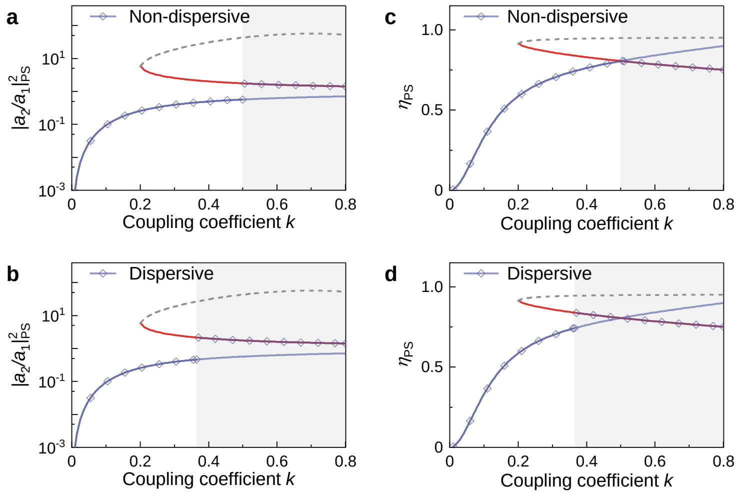


**Fig. S5 Performance of parallel-series (PS) topology circuits using dispersive and non-dispersive gain. a,b** Energy storage ratio and **c,d** efficiency of non-dispersive and dispersive PT-symmetric WPT system with PS topology as a function of the coupling parameter $k$ when $\chi = 4/3$.

# 3 Design and characterization of dispersion-gain-based WPT system

## 3.1 Design of the dispersive gain element

Negative resistors are commonly used as gain elements in PT-symmetric WPT systems. Unlike the usual resistors, negative resistors can produce a negative current proportional to a positive voltage applied to their terminals. The common negative resistor is frequency independent. However, by applying the frequency dispersion phenomenon such as the skin effect of actual resistors, negative resistors can also be frequency-dependent. Here, we attempt to introduce frequency-dependent negative resistors, i.e., dispersive gain devices, into the non-Hermitian systems. In particular, we use a generalized impedance converter (GIC) to construct a frequency-dependent negative resistor [10], as shown in the pink shaded region of the circuit given in Fig. S6**a**. In the case of a sinusoidal steady state, the equivalent impedance of the GIC is

$$Z_{\mathrm{eq}} = \frac{R_{\mathrm{f1}} R_{\mathrm{f2}} R_{\mathrm{g}}}{\frac{1}{\mathrm{i}\omega C_{\mathrm{f1}}} \frac{1}{\mathrm{i}\omega C_{\mathrm{f2}}}} = -\omega^2 R_{\mathrm{eq}}, \tag{S14}$$

which is a frequency-dependent (dispersive) negative resistance proportional to $\omega^2$. Fig. S6**b** compares the simulated static $I$–$V$ curves of the dispersive negative resistor and the traditional saturated negative resistor. As a reference, a schematic diagram of a commonly used negative resistor with saturation characteristics is also illustrated in Fig. S6**b**, which stems from the limited output of the integrated operational amplifier and has been extensively analyzed. The inset of Fig. S6**b** shows the AC $I$–$V$ curve at the design frequency of 1.3 MHz. For the conventional negative resistor, there is a section of the $I$–$V$ curve that has a negative slope, which shows negative resistance characteristics. In contrast, the dispersive negative resistor only serves as negative resistance under AC conditions.

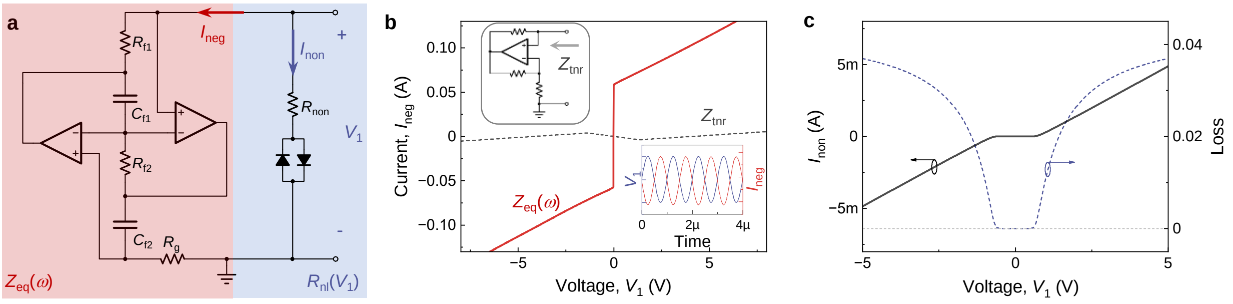


**Fig. S6 Design of the dispersive gain element with nonlinear behavior. a** Schematic and **b,c** characteristics of our dispersive nonlinear gain element. **b**, Comparison of the simulated behavior between the dispersive nonlinear gain element and the traditional saturated gain element. In **b**, the black dash line is simulation result of the traditional saturation gain element. **c**, Simulated nonlinear behavior of the nonlinear resistor.

Due to the breaking of the PT symmetry, the required gain varies under different coupling coefficients to maintain a steady state. To achieve robust wireless power transfer without tuning [4], it is necessary to introduce nonlinearity into the gain component to achieve dynamic gain-loss balance. In the traditional design of negative resistors, we can directly utilize the saturation characteristics of operational amplifiers to achieve this balance [9]. However, since two integrated operational amplifiers are used in the dispersive gain device based on the GIC, the saturation characteristics become very complex considering the non-ideal factors of active devices. To achieve a controllable saturation behavior, we parallel the GIC with a nonlinear resistor composed of a resistor and anti-parallel diodes, as shown in the blue-shaded region in Fig. S6**a**, whose equivalent resistance is a function of voltage, i.e., $R_{\mathrm{nl}} = R_{\mathrm{nl}}(V_1)$. In our design, since the nonlinear resistor saturates earlier than the operational amplifier, the parameter $g_c$ is approximately a constant value of $g_{\mathrm{nl}}(V_1,\omega) = g_{\mathrm{c}}/\omega^2 - \gamma_{\mathrm{nl}}(V_1)$, and the nonlinear loss $\gamma_{\mathrm{nl}}(V_1) = Z_{\mathrm{r}}/R_{\mathrm{nl}}(V_1)$ changes adaptively to maintain the steady-state mode. The loss tends to increase as the voltage increases because the diode in the nonlinear resistor makes the equivalent resistance smaller (see Fig. S6**c**). Due to the voltage-limiting effect of the antiparalleled diode, the frequency-domain negative resistor is anchored in the linear region to avoid complex saturation behavior. Moreover, we can utilize the nonlinearity between the loss of the nonlinear resistor and the voltage amplitude to achieve dynamic gain-loss balance. Although new losses in the gain element may be introduced, our design enables verification of the dispersive WPT system at a low cost. When designing practical WPT systems, the construction of a dispersive gain source without nonlinear source by digital control or fractional order control may further achieve a high-efficiency system.

### 3.2 Design of the asymmetric wireless power transfer system

Although both the asymmetry of the circuit topology and the dispersive gain can induce mode-switching phenomena, the output characteristics of different topologies are significantly different. We can achieve the desired high efficiency and output characteristics by adjusting circuit parameters. For magnetically coupled WPT systems, changing the resonant parameters by adjusting the compensation capacitor is more feasible because replacing capacitive components or adjusting variable capacitor parameters will not affect the magnetic coupling coefficient. Thus, the asymmetry parameter $\chi$ can be adjusted by varying the capacitance. Compared to the PT-symmetric system, more energy is concentrated in the receiver resonator for the asymmetric system, indicating that the efficiency of the system is more sensitive to the inherent loss of the load-side coil than that of the source-side coil. To our knowledge, the implementation of high-quality series compensation coils is more feasible and can effectively raise the power capacity, while negative resistance based on the operational amplifier circuit is usually more suitable for parallel resonant circuits due to the existence of hidden poles [11]. Therefore, we have designed a parallel-series prototype circuit as a practical design reference.

The experimental prototype circuit is shown in Fig. S7. The detailed circuit board layout is shown in Fig. S8. Here, $R_{\mathrm{sp}}$ is the equivalent parallel resistance of the intrinsic loss of the source side resonator, $R_{\mathrm{rs}}$ is the parasitic resistance of the receiving resonator, and $R_{\mathrm{ls}}$ is the load resistance. The corresponding loss coefficients are $\gamma_{\mathrm{s}} = Z_{\mathrm{r}}/R_{\mathrm{sp}}$, $\gamma_r = R_{\mathrm{rs}}/Z_{\mathrm{r}}$, and $\gamma_{\mathrm{load}} = R_{\mathrm{ls}}/Z_{\mathrm{r}}$. A pair of 10-cm-diameter coils wound with different Litz wires is used as the system's coupling link. The receiving coil is configured as a series *RLC* resonator with a natural resonant frequency ($\omega_{\mathrm{n}2}/2\pi$) of 1.53 MHz and a measured quality factor ($1/\gamma$) of 5.23 by a load resistance of about 2 Ω. In contrast, the source coil is configured as a parallel resonance with a resonant frequency ($\omega_{\mathrm{n}1}/2\pi$) of 1.31 MHz. The intrinsic quality factors measured for the source and load *LC* resonators are $Q_{\mathrm{s}} \approx 72$ and $Q_{\mathrm{r}} \approx 268$, respectively. A dual channel operational amplifier LT1813 is configured as a generalized impedance converter and functions as a dispersive gain element with an adjustable resistor of $R_{\mathrm{g}} \approx 80\ \Omega$. Two coils are placed coaxially on a rail and the coupling coefficient $k$ can be adjusted by changing the separation distance $d$. Fig. S9 shows the relationship between the measured coupling coefficient and the coaxial distance of the coil. To minimize the impact of the nonideal factors of the op-amp on the gain element's output characteristics, the ground resistance $R_{\mathrm{g}}$ should be chosen to ensure that the voltage and current of the negative resistance element are in phase.

## 4 Mode selection mechanism

In determining the steady-state mode of a nonlinear multimode system, the most common approach is based on Lyapunov methods, whose feasibility is dictated by the precise modeling of nonlinear components. However, for real-world systems, it remains a challenge to quantify and model various types of nonlinear devices accurately. A qualitative analysis approach may be more useful to explore mode selection mechanisms. By utilizing the qualitative method, we can investigate the steady-state mechanisms of systems contaning novel devices that have never been modeled, accelerating the development and design process of novel types of nonlinear systems. Here, we apply the qualitative analysis method used previously [4, 9, 12] to demonstrate the mode selection mechanism of our nonlinear multimode systems. More specifically, we ignore the precise mathematical modeling of nonlinear devices and instead capture their essential physical properties. For example, it has been previously observed [3, 4, 13–17] that for gain-saturated devices, the equivalent gain of saturated gain devices would decrease as the extent of saturation increases. Therefore, we can follow the lowest-gain principle to determine the steady-state mode, i.e., the mode requiring the minimum gain among multiple theoretical modes is the steady-state mode.

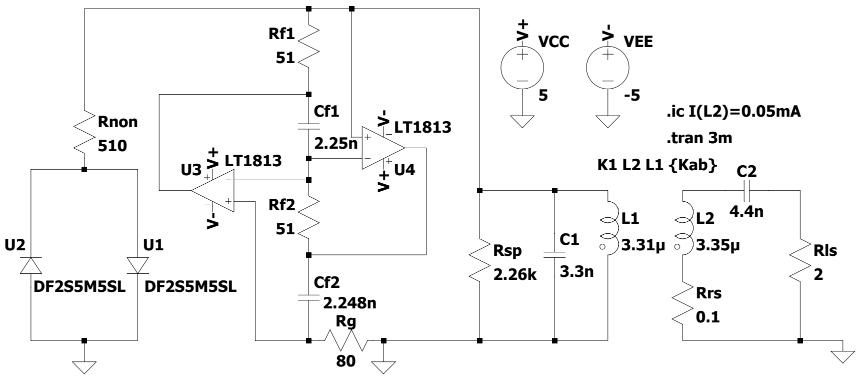


**Fig. S7 Circuit diagram of the experimental prototype.**

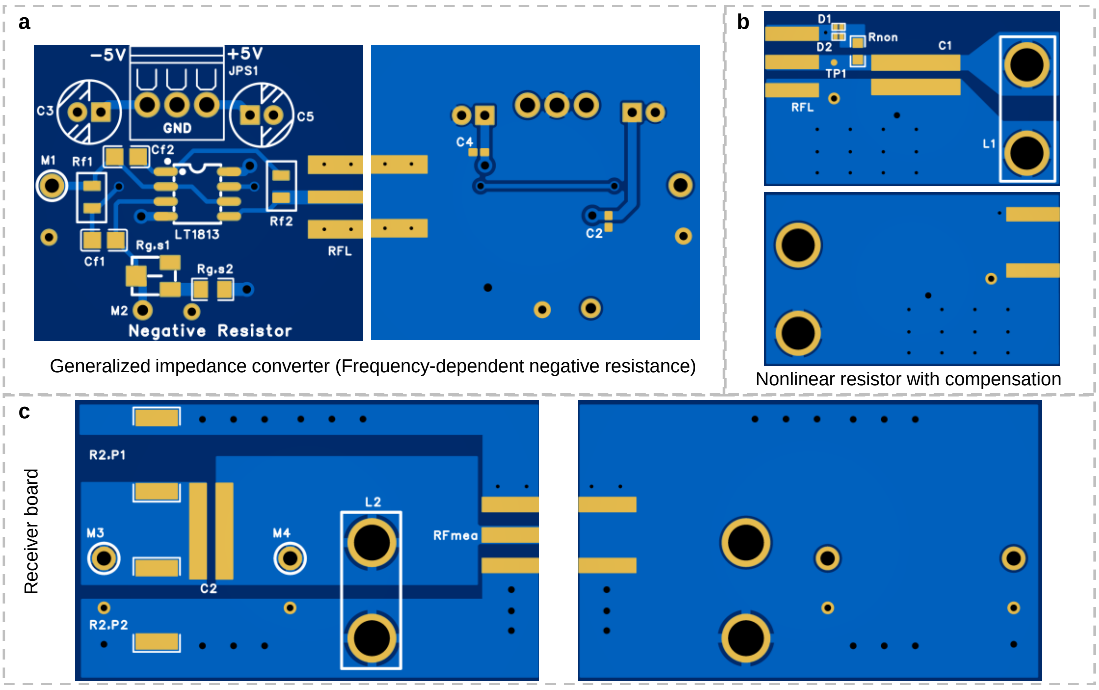


**Fig. S8 Layout of the experimental circuit. a** Dispersive gain element and **b** nonlinear resistor with compensation constitute the source circuit board. **c** Receive circuit board configured as a series *RLC* circuit.

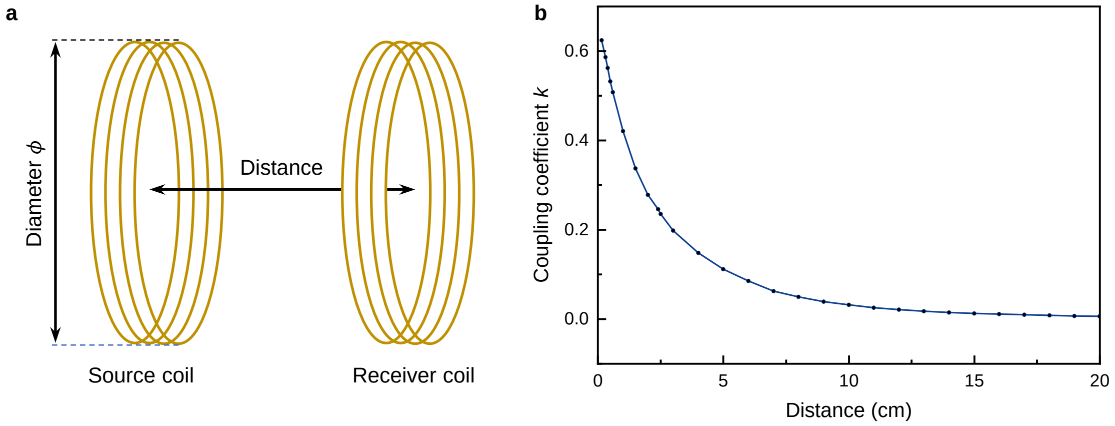


**Fig. S9 Design of wireless power transfer coils. a**, The schematic and parameter of the coils. **b**, Coupling coefficients $k$ with respect to the distance between the source and receiver coils.

When discussing the ideal saturation-type dispersive gain $g_{\mathrm{nl}}(V_1, \omega) = g_{\mathrm{src}}(V_1)/\omega^2$, we assume that $g_{\mathrm{src}}(V_1)$ is a nonlinear gain that tends to be minimal. For the proposed nonlinear dispersive gain element that is composed of nonlinear resistors and frequency-dependent negative resistors, the characteristics of the nonlinear resistor determine the saturation features of the entire component since the frequency-dependent negative resistor operates in the linear region. As shown in Fig. S6**c**, in the saturation region, the loss of the nonlinear resistor tends to increase as the voltage increases. Therefore, the mode-selection mechanism of the system based on this component can be based on the principle of maximum nonlinear loss, i.e., the mode requiring the maximum nonlinear loss is the steady-state mode.

Note that above analytical principles are directed towards global steady-state scenarios. For multistable regions, although the steady-state mechanisms are more complex, a qualitative physical interpretation can still be provided. Fig. S10 illustrates the spectrum of the loss required in the steady state in different parameter regions of the asymmetric system. As mentioned above, one can qualitatively assess the stability based on the characteristics of nonlinear devices. Since the loss rate of nonlinear resistors is always positive, the mode is stable as long as the required loss is positive. Depending on the gain and loss parameters, the theoretically supported modes of the system can fall into three categories: bistable (Fig. S10**a**), monostable (Fig. S10**b,c**), and zero-stable (Fig. S10**d**). When the system is turned on from a zero initial condition, the steady-state mechanism follows the principle of maximum loss. However, in bistable scenarios, if the initial condition is near one of the system's steady states, the system will be attracted to these local steady states rather than evolving towards the global steady state with the maximum required loss, which leads to an asymmetric hysteretic mode switching phenomenon. In summary, a graphical approach based on qualitative analysis can be provided for steady-state selection. More specific and detailed analysis of the basins of attraction and dynamic characteristics may require precise mathematical modeling of nonlinear devices.

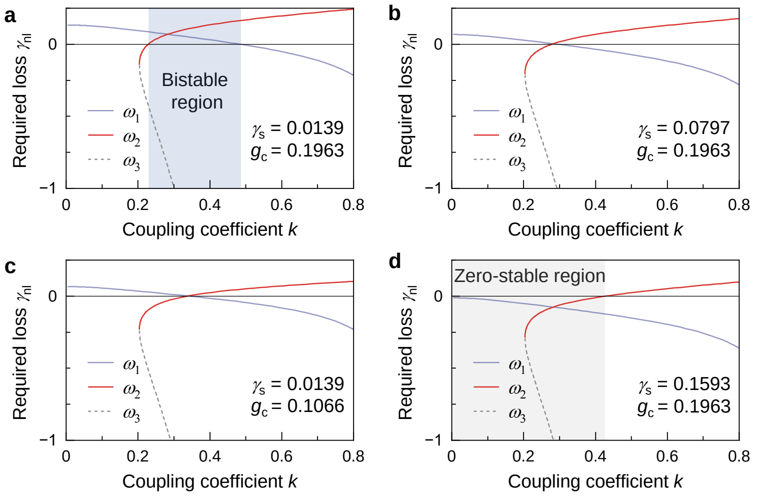


**Fig. S10 Computed steady-state required loss spectrum of three modes for different gain $g_c$ and loss $\gamma_s$ parameter a**, Loss spectrum including the bistable region; **b,c**, Loss spectrum of only the monostable region; **d**, Loss spectrum including the zero-stable region.

# References


[1] Haus, H. A. *Waves and fields in optoelectronics* (Prentice Hall, Hoboken, NJ, USA, 1984).

[2] Kurs, A. *et al.* Wireless power transfer via strongly coupled magnetic resonances. *Science* **317**, 83–86 (2007).

[3] Assawaworrarit, S. & Fan, S. Robust and efficient wireless power transfer using a switch-mode implementation of a nonlinear parity–time symmetric circuit. *Nature Electronics* **3**, 273–279 (2020).

[4] Assawaworrarit, S., Yu, X. & Fan, S. Robust wireless power transfer using a nonlinear parity–time-symmetric circuit. *Nature* **546**, 387–390 (2017).

[5] Wu, J., Li, K., Zeng, J. & Hui, S.-Y. R. On the limitations of the coupled mode theory and parity-time symmetry for near-field wireless power transfer research. *IEEE Transactions on Power Electronics* **39**, 6433–6441 (2024).

[6] Schindler, J., Li, A., Zheng, M. C., Ellis, F. M. & Kottos, T. Experimental study of active LRC circuits with PT symmetries. *Physical Review A* **84**, 040101 (2011).

[7] Dong, Z., Li, Z., Yang, F., Qiu, C.-W. & Ho, J. S. Sensitive readout of implantable microsensors using a wireless system locked to an exceptional point. *Nature Electronics* **2**, 335–342 (2019).

[8] Sakhdari, M., Hajizadegan, M. & Chen, P.-Y. Robust extended-range wireless power transfer using a higher-order PT-symmetric platform. *Physical Review Research* **2**, 013152 (2020).

[9] Hao, X. *et al.* Frequency-stable robust wireless power transfer based on high-order pseudo-Hermitian physics. *Physical Review Letters* **130**, 077202 (2023).

[10] Mishonov, T. M., Dimitrova, I. M., Serafimov, N. S., Petkov, E. G. & Varonov, A. M. Q-factor of the resonators with frequency dependent negative resistor. *IEEE Transactions on Circuits and Systems II: Express Briefs* **69**, 694–698 (2021).

[11] Schindler, J. *et al.* PT-symmetric electronics. *Journal of Physics A: Mathematical and Theoretical* **45**, 444029 (2012).

[12] Yin, K. *et al.* Wireless real-time capacitance readout based on perturbed nonlinear parity-time symmetry. *Applied Physics Letters* **120**, 194101 (2022).

[13] Zhou, J., Zhang, B., Xiao, W., Qiu, D. & Chen, Y. Nonlinear parity-time-symmetric model for constant efficiency wireless power transfer: Application to a drone-in-flight wireless charging platform. *IEEE Transactions on Industrial Electronics* **66**, 4097–4107 (2018).

[14] Suntharalingam, A., Fernández-Alcázar, L., Kononchuk, R. & Kottos, T. Noise resilient exceptional-point voltmeters enabled by oscillation quenching phenomena. *Nature Communications* **14**, 5515 (2023).

[15] Hua, Z., Chau, K., Liu, W., Tian, X. & Pang, H. Autonomous pulse frequency modulation for wireless battery charging with zero-voltage switching. *IEEE Transactions on Industrial Electronics* **70**, 8959–8969 (2022).

[16] Bai, K. *et al.* Nonlinearity-enabled higher-order exceptional singularities with ultra-enhanced signal-to-noise ratio. *National Science Review* **10**, nwac259 (2023).

[17] Bai, K. *et al.* Observation of nonlinear exceptional points with a complete basis in dynamics. *Physical Review Letters* **132**, 073802 (2024).

Dated: July 22, 2024
